# Supplementary material for: Microscopic Mechanism of the Thermal Amorphization of ZIF-4 and Melting of ZIF-zni Revealed via Molecular Dynamics and Machine Learning Techniques
Source: arXiv:2311.16351 source file (2023-11-27)
Supplement: Supplementary file 1 [file Thermal_Amorphisation_of_ZIF_4_and_ZIF_zni__arXiv_SM.pdf]

Supplementary Material for:

# Microscopic Mechanism of the Thermal Amorphization of ZIF-4 and Melting of ZIF-zni Revealed via Molecular Dynamics and Machine Learning Techniques

Emilio Mendez[1] and Rocio Semino[1]

*Sorbonne Université, CNRS, Physico-chimie des Electrolytes et Nanosystèmes Interfaciaux, PHENIX, F-75005 Paris, France*

(*Electronic mail: rocio.semino@sorbonne-universite.fr)

## CONTENTS

**I. Generation of the Amorphous Structures** 2

**II. Machine Learning Methods** 2

**III. Thermodynamic Analyses** 4

**IV. Mechanisms of the Phase Transitions** 5

**References** 6

# I. GENERATION OF THE AMORPHOUS STRUCTURES

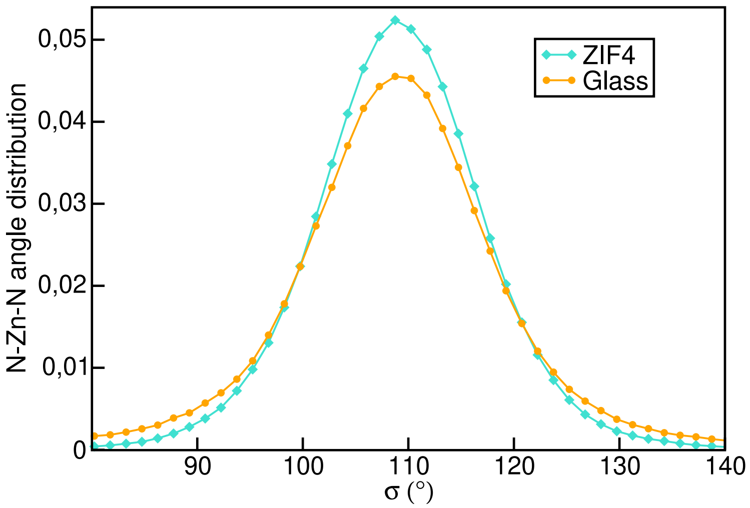


Fig. S 1. ZIF-4 (light blue) and ZIF_a (orange) N–Zn–N angle distribution computed *via* nb-ZIF-FF.

# II. MACHINE LEARNING METHODS

**Symmetry Functions:** The values of $\eta$ for the radial functions are 0.005, 0.0075, 0.01 and 0.02 Bohr$^{-2}$. With each of these $\eta$ values, we construct two angular functions with $\lambda$=$\pm$1. In all cases $R_s$ was set to zero and $\zeta$ was set to one. The cutoff radius $R_c$ was set to $\sim$ 13 Å, comprising approximately the first two coordination shells. The symmetry functions were normalised so that the highest and lowest values in the database were assigned one and zero respectively.

**Neural Network:** The training of the neural network was done using the R software in conjunction with Keras package.[?] Rectified linear activation functions were employed for the hidden layer while the softmax function was used for the output layer. The categorical cross-entropy was selected as loss function to be minimised.[?] We employed the Adam algorithm for the optimisation of the neural network parameters. This process was done over 350 epochs of the training set.

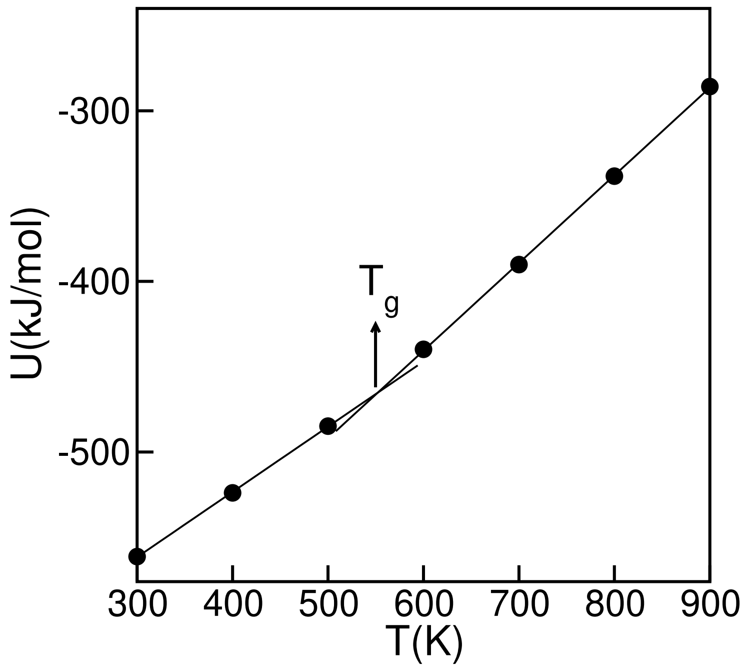


Fig. S 2. Average potential energy as a function of temperature (black dots). Lines correspond to linear regressions of the points above/below $T_g$.

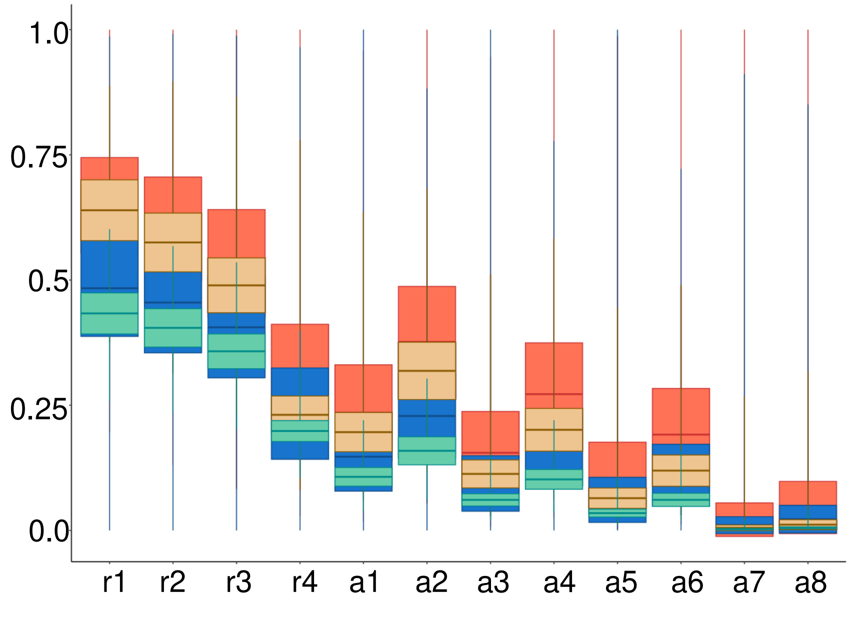


Fig. S 3. Box plots depicting the statistical distribution of the normalised symmetry functions in the data set: ZIF-4 (green), ZIF-zni (orange), ZIF_a (red), and ZIF_liq (blue). The boxes sizes correspond to twice the standard deviations. The upper and lower lines indicate maximum and minimum values respectively. r*i* with *i*=1-4 correspond to the four radial symmetry functions considered while a*i* with *i*=1-8 correspond to the eight angular ones.

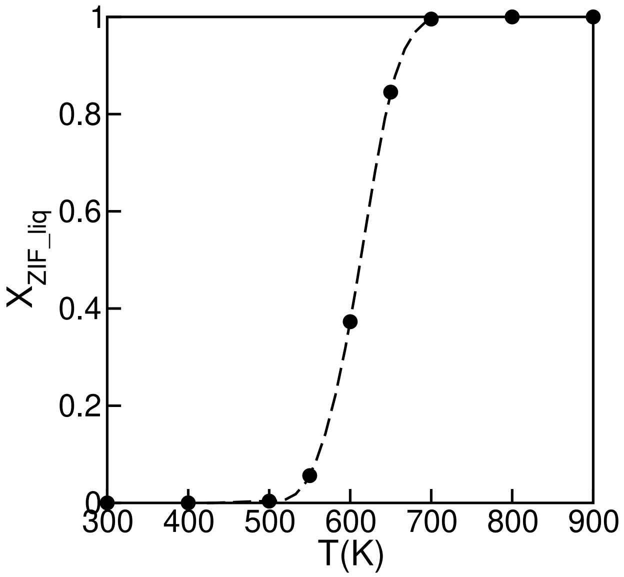


Fig. S 4. Fraction of disordered $Zn^{2+}$ centres classified as ZIF_liq as a function of temperature.

## III. THERMODYNAMIC ANALYSES

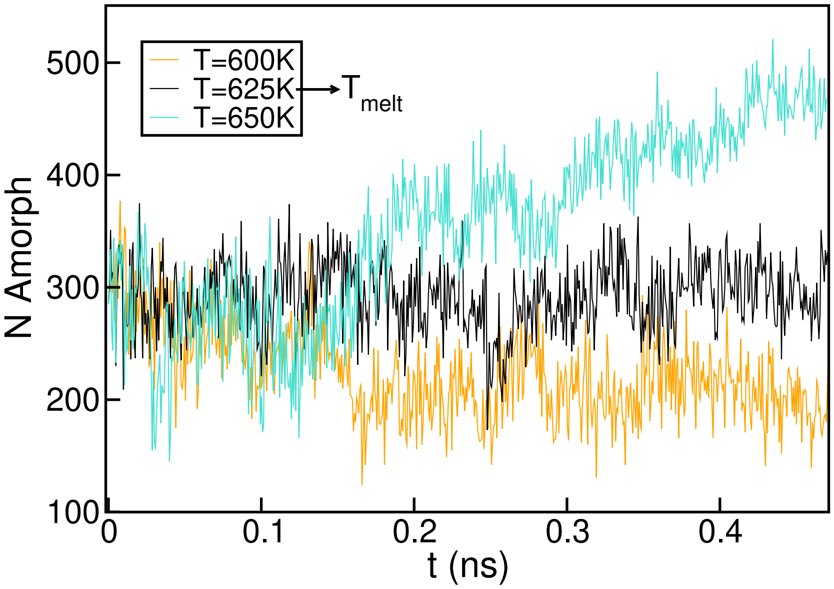


Fig. S 5. Time evolution of the number of disordered (ZIF_a-like or ZIF_liq-like) $Zn^{2+}$ centres for NPT simulations that differ in the constant target temperature in a simulation that starts from an initial microstate where half of the centres are ordered (ZIF-zni) and the other half disordered.

## IV. MECHANISMS OF THE PHASE TRANSITIONS

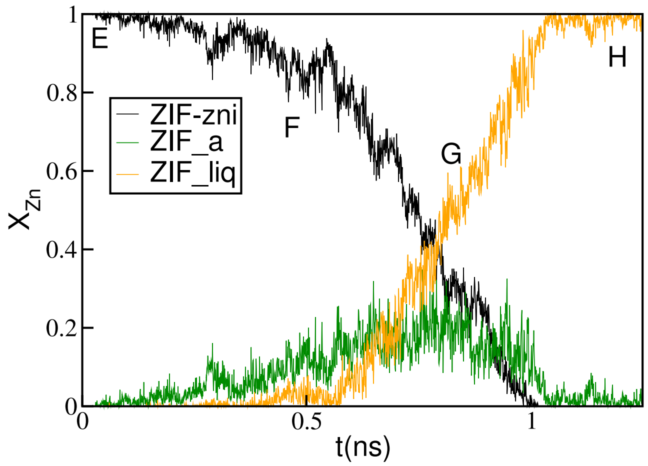


Fig. S 6. Time evolution of the number of disordered (amorphous- and liquid-like) $Zn^{2+}$ centres for a melting simulation starting from a ZIF-zni crystal.

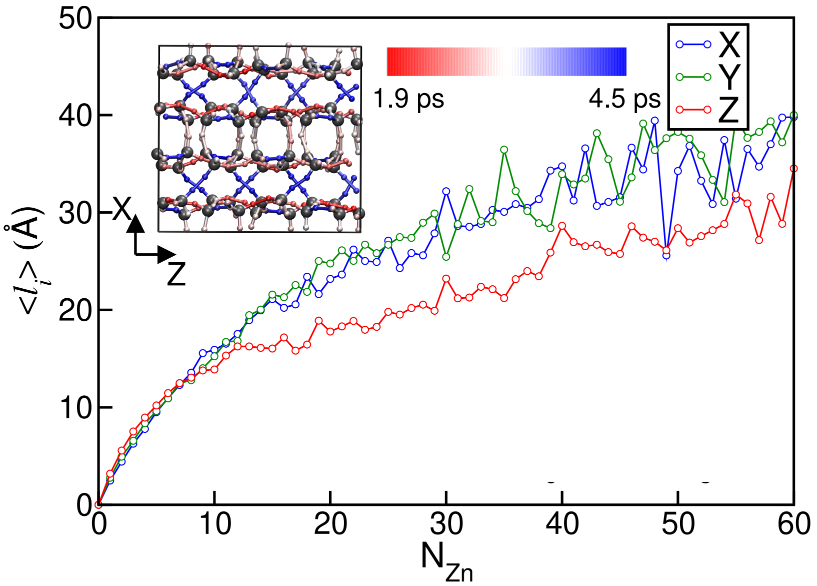


Fig. S 7. Average length in each of the three cartesian axes directions as a function of $N_{Zn}$, the number of $Zn^{2+}$ centres in the ZIF_a cluster along ZIF-zni melting. The inset shows a snapshot of the unit cell in the XZ plane. Each ligand is coloured according to its tendency for bond breaking. The colour scale is related to the average time associated to the bond breaking process: from red (less stable bonds) to blue (more stable) passing through white (intermediate reactivity bonds). Only N and $Zn^{2+}$ atoms (grey) are shown.

# REFERENCES

[1]S. Horike, S. S. Nagarkar, T. Ogawa, and S. Kitagawa, "A new dimension for coordination polymers and metal–organic frameworks: Towards functional glasses and liquids," Angewandte Chemie International Edition **59**, 6652–6664 (2020).

[2]A. W. Thornton, K. E. Jelfs, K. Konstas, C. M. Doherty, A. J. Hill, A. K. Cheetham, and T. D. Bennett, "Porosity in metal–organic framework glasses," Chemical Communications **52**, 3750–3753 (2016).

[3]N. Ma and S. Horike, "Metal–organic network-forming glasses," Chemical Reviews **122**, 4163–4203 (2022).

[4]J. Fonseca, T. Gong, L. Jiao, and H.-L. Jiang, "Metal–organic frameworks (MOFs) beyond crystallinity: amorphous MOFs, MOF liquids and MOF glasses," Journal of Materials Chemistry A **9**, 10562–10611 (2021).

[5]T. Zhang, J. Wang, W. Zhang, C. Yang, L. Zhang, W. Zhu, J. Sun, G. Li, T. Li, and J. Wang, "Amorphous fe/mn bimetal–organic frameworks: outer and inner structural designs for efficient arsenic(scpiii/scp) removal," Journal of Materials Chemistry A **7**, 2845–2854 (2019).

[6]C. Orellana-Tavra, R. J. Marshall, E. F. Baxter, I. A. Lázaro, A. Tao, A. K. Cheetham, R. S. Forgan, and D. Fairen-Jimenez, "Drug delivery and controlled release from biocompatible metal–organic frameworks using mechanical amorphization," Journal of Materials Chemistry B **4**, 7697–7707 (2016).

[7]C. Orellana-Tavra, M. Köppen, A. Li, N. Stock, and D. Fairen-Jimenez, "Biocompatible, crystalline, and amorphous bismuth-based metal–organic frameworks for drug delivery," ACS Applied Materials &amp Interfaces **12**, 5633–5641 (2020).

[8]D. F. Sava, M. A. Rodriguez, K. W. Chapman, P. J. Chupas, J. A. Greathouse, P. S. Crozier, and T. M. Nenoff, "Capture of volatile iodine, a gaseous fission product, by zeolitic imidazolate framework-8," Journal of the American Chemical Society **133**, 12398–12401 (2011).

[9]K. W. Chapman, D. F. Sava, G. J. Halder, P. J. Chupas, and T. M. Nenoff, "Trapping guests within a nanoporous metal–organic framework through pressure-induced amorphization," Journal of the American Chemical Society **133**, 18583–18585 (2011).

[10]B. Yu, J. Hou, and J. Gong, "Amorphous co(MeIm)sub2/sub framework coating on AuCo for size-selective photocatalysis and interface transfer," Catal. Sci. Technol. **7**, 5004–5010 (2017).

[11]Y. Duan, Z.-Y. Yu, S.-J. Hu, X.-S. Zheng, C.-T. Zhang, H.-H. Ding, B.-C. Hu, Q.-Q. Fu, Z.-

L. Yu, X. Zheng, J.-F. Zhu, M.-R. Gao, and S.-H. Yu, "Scaled-up synthesis of amorphous NiFeMo oxides and their rapid surface reconstruction for superior oxygen evolution catalysis," Angewandte Chemie International Edition **58**, 15772–15777 (2019).

[12]D. Bazer-Bachi, L. Assié, V. Lecocq, B. Harbuzaru, and V. Falk, "Towards industrial use of metal-organic framework: Impact of shaping on the MOF properties," Powder Technology **255**, 52–59 (2014).

[13]J. C. Tan, T. D. Bennett, and A. K. Cheetham, "Chemical structure, network topology, and porosity effects on the mechanical properties of zeolitic imidazolate frameworks," Proceedings of the National Academy of Sciences **107**, 9938–9943 (2010).

[14]G. N. Greaves, F. Meneau, A. Sapelkin, L. M. Colyer, I. ap Gwynn, S. Wade, and G. Sankar, "The rheology of collapsing zeolites amorphized by temperature and pressure," Nature Materials **2**, 622–629 (2003).

[15]I. Peral and J. Íñiguez, "Amorphization induced by pressure: Results for zeolites and general implications," Physical Review Letters **97** (2006), 10.1103/physrevlett.97.225502.

[16]T. D. Bennett, A. L. Goodwin, M. T. Dove, D. A. Keen, M. G. Tucker, E. R. Barney, A. K. Soper, E. G. Bithell, J.-C. Tan, and A. K. Cheetham, "Structure and properties of an amorphous metal-organic framework," Physical Review Letters **104** (2010), 10.1103/physrevlett.104.115503.

[17]T. D. Bennett, D. A. Keen, J.-C. Tan, E. R. Barney, A. L. Goodwin, and A. K. Cheetham, "Thermal amorphization of zeolitic imidazolate frameworks," Angewandte Chemie International Edition **50**, 3067–3071 (2011).

[18]T. D. Bennett, P. Simoncic, S. A. Moggach, F. Gozzo, P. Macchi, D. A. Keen, J.-C. Tan, and A. K. Cheetham, "Reversible pressure-induced amorphization of a zeolitic imidazolate framework (ZIF-4)," Chemical Communications **47**, 7983 (2011).

[19]T. D. Bennett, S. Cao, J. C. Tan, D. A. Keen, E. G. Bithell, P. J. Beldon, T. Friscic, and A. K. Cheetham, "Facile mechanosynthesis of amorphous zeolitic imidazolate frameworks," Journal of the American Chemical Society **133**, 14546–14549 (2011).

[20]R. N. Widmer, G. I. Lampronti, N. Casati, S. Farsang, T. D. Bennett, and S. A. T. Redfern, "X-ray radiation-induced amorphization of metal–organic frameworks," Physical Chemistry Chemical Physics **21**, 12389–12395 (2019).

[21]J.-B. Weiß and S. Henke, "Forging links in molecular glasses," Nature Synthesis (2023), 10.1038/s44160-023-00425-0.

[22]N. Masciocchi, S. Bruni, E. Cariati, F. Cariati, S. Galli, and A. Sironi, "Extended polymor-

phism in copper(II) imidazolate polymers: a spectroscopic and XRPD structural study," Inorganic Chemistry **40**, 5897–5905 (2001).

[23]K. Ohara, J. Martí-Rujas, T. Haneda, M. Kawano, D. Hashizume, F. Izumi, and M. Fujita, "Formation of a thermally stable, porous coordination network via a crystalline-to-amorphous-to-crystalline phase transition," Journal of the American Chemical Society **131**, 3860–3861 (2009).

[24]L. León-Alcaide, R. S. Christensen, D. A. Keen, J. L. Jordá, I. Brotons-Alcázar, A. Forment-Aliaga, and G. M. Espallargas, "Meltable, glass-forming, iron zeolitic imidazolate frameworks," Journal of the American Chemical Society **145**, 11258–11264 (2023).

[25]M. Hartmann, U. Böhme, M. Hovestadt, and C. Paula, "Adsorptive separation of olefin/paraffin mixtures with ZIF-4," Langmuir **31**, 12382–12389 (2015).

[26]M. Hovestadt, J. V. Schmitz, T. Weissenberger, F. Reif, M. Kaspereit, W. Schwieger, and M. Hartmann, "Scale-up of the synthesis of zeolitic imidazolate framework ZIF-4," Chemie Ingenieur Technik **89**, 1374–1378 (2017).

[27]K. S. Park, Z. Ni, A. P. Côté, J. Y. Choi, R. Huang, F. J. Uribe-Romo, H. K. Chae, M. O'Keeffe, and O. M. Yaghi, "Exceptional chemical and thermal stability of zeolitic imidazolate frameworks," Proceedings of the National Academy of Sciences **103**, 10186–10191 (2006).

[28]R. N. Widmer, G. I. Lampronti, S. Chibani, C. W. Wilson, S. Anzellini, S. Farsang, A. K. Kleppe, N. P. M. Casati, S. G. MacLeod, S. A. T. Redfern, F.-X. Coudert, and T. D. Bennett, "Rich polymorphism of a metal–organic framework in pressure–temperature space," Journal of the American Chemical Society **141**, 9330–9337 (2019).

[29]T. D. Bennett, Y. Yue, P. Li, A. Qiao, H. Tao, N. G. Greaves, T. Richards, G. I. Lampronti, S. A. T. Redfern, F. Blanc, O. K. Farha, J. T. Hupp, A. K. Cheetham, and D. A. Keen, "Melt-quenched glasses of metal–organic frameworks," Journal of the American Chemical Society **138**, 3484–3492 (2016).

[30]E. O. R. Beake, M. T. Dove, A. E. Phillips, D. A. Keen, M. G. Tucker, A. L. Goodwin, T. D. Bennett, and A. K. Cheetham, "Flexibility of zeolitic imidazolate framework structures studied by neutron total scattering and the reverse monte carlo method," Journal of Physics: Condensed Matter **25**, 395403 (2013).

[31]T. D. Bennett, J.-C. Tan, Y. Yue, E. Baxter, C. Ducati, N. J. Terrill, H. H. M. Yeung, Z. Zhou, W. Chen, S. Henke, A. K. Cheetham, and G. N. Greaves, "Hybrid glasses from strong and fragile metal-organic framework liquids," Nature Communications **6** (2015), 10.1038/ncomms9079.

[32]E. F. Baxter, T. D. Bennett, C. Mellot-Draznieks, C. Gervais, F. Blanc, and A. K. Cheetham,

"Combined experimental and computational NMR study of crystalline and amorphous zeolitic imidazolate frameworks," Physical Chemistry Chemical Physics **17**, 25191–25196 (2015).

[33]M. R. Ryder, T. D. Bennett, C. S. Kelley, M. D. Frogley, G. Cinque, and J.-C. Tan, "Tracking thermal-induced amorphization of a zeolitic imidazolate framework via synchrotron in situ far-infrared spectroscopy," Chemical Communications **53**, 7041–7044 (2017).

[34]R. Gaillac, P. Pullumbi, K. A. Beyer, K. W. Chapman, D. A. Keen, T. D. Bennett, and F.-X. Coudert, "Liquid metal–organic frameworks," Nature Materials **16**, 1149–1154 (2017).

[35]R. Gaillac, P. Pullumbi, and F.-X. Coudert, "Melting of zeolitic imidazolate frameworks with different topologies: Insight from first-principles molecular dynamics," The Journal of Physical Chemistry C **122**, 6730–6736 (2018).

[36]Y. Yang, Y. K. Shin, S. Li, T. D. Bennett, A. C. T. van Duin, and J. C. Mauro, "Enabling computational design of ZIFs using ReaxFF," The Journal of Physical Chemistry B **122**, 9616–9624 (2018).

[37]N. Castel and F.-X. Coudert, "Challenges in molecular dynamics of amorphous ZIFs using reactive force fields," The Journal of Physical Chemistry C **126**, 19532–19541 (2022).

[38]S. R. G. Balestra and R. Semino, "Computer simulation of the early stages of self-assembly and thermal decomposition of ZIF-8," The Journal of Chemical Physics **157** (2022), 10.1063/5.0128656.

[39]C. R. Groom, I. J. Bruno, M. P. Lightfoot, and S. C. Ward, "The cambridge structural database," Acta Crystallographica Section B Structural Science, Crystal Engineering and Materials **72**, 171–179 (2016).

[40]N. Castel and F.-X. Coudert, "Computation of finite temperature mechanical properties of zeolitic imidazolate framework glasses by molecular dynamics," Chemistry of Materials **35**, 4038–4047 (2023).

[41]A. F. Sapnik, C. Sun, J. E. M. Laulainen, D. N. Johnstone, R. Brydson, T. Johnson, P. A. Midgley, T. D. Bennett, and S. M. Collins, "Mapping nanocrystalline disorder within an amorphous metal–organic framework," Communications Chemistry **6** (2023), 10.1038/s42004-023-00891-9.

[42]N. C. Karayiannis, K. Foteinopoulou, and M. Laso, "The characteristic crystallographic element norm: A descriptor of local structure in atomistic and particulate systems," The Journal of Chemical Physics **130** (2009), 10.1063/1.3077294.

[43]F. Pietrucci and R. Martoňák, "Systematic comparison of crystalline and amorphous phases:

Charting the landscape of water structures and transformations," The Journal of Chemical Physics **142** (2015), 10.1063/1.4914138.

[44]M. A. Caro, A. Aarva, V. L. Deringer, G. Csányi, and T. Laurila, "Reactivity of amorphous carbon surfaces: Rationalizing the role of structural motifs in functionalization using machine learning," Chemistry of Materials **30**, 7446–7455 (2018).

[45]K. Swanson, S. Trivedi, J. Lequieu, K. Swanson, and R. Kondor, "Deep learning for automated classification and characterization of amorphous materials," Soft Matter **16**, 435–446 (2020).

[46]S. Banik, D. Dhabal, H. Chan, S. Manna, M. Cherukara, V. Molinero, and S. K. R. S. Sankaranarayanan, "CEGANN: Crystal edge graph attention neural network for multiscale classification of materials environment," npj Computational Materials **9** (2023), 10.1038/s41524-023-00975-z.

[47]J. Rogal, E. Schneider, and M. E. Tuckerman, "Neural-network-based path collective variables for enhanced sampling of phase transformations," Physical Review Letters **123** (2019), 10.1103/physrevlett.123.245701.

[48]J. Behler, "Atom-centered symmetry functions for constructing high-dimensional neural network potentials," The Journal of Chemical Physics **134** (2011), 10.1063/1.3553717.

[49]J. Behler, "Constructing high-dimensional neural network potentials: A tutorial review," International Journal of Quantum Chemistry **115**, 1032–1050 (2015).

[50]R Core Team, *R: A Language and Environment for Statistical Computing*, R Foundation for Statistical Computing, Vienna, Austria (2022).

[51]S. S. Schoenholz, E. D. Cubuk, D. M. Sussman, E. Kaxiras, and A. J. Liu, "A structural approach to relaxation in glassy liquids," Nature Physics **12**, 469–471 (2016).

[52]A. P. Thompson, H. M. Aktulga, R. Berger, D. S. Bolintineanu, W. M. Brown, P. S. Crozier, P. J. in 't Veld, A. Kohlmeyer, S. G. Moore, T. D. Nguyen, R. Shan, M. J. Stevens, J. Tranchida, C. Trott, and S. J. Plimpton, "LAMMPS - a flexible simulation tool for particle-based materials modeling at the atomic, meso, and continuum scales," Computer Physics Communications **271**, 108171 (2022).

[53]K. Govers, S. Lemehov, M. Hou, and M. Verwerft, "Comparison of interatomic potentials for uo2," Journal of Nuclear Materials **376**, 66–77 (2008).
